# Supplementary material for: Resolving Word Vagueness with Scenario-guided Adapter for Natural Language Inference
Source: arXiv:2405.12434 source file (2024-05-21)
Supplement: Supplementary file 1 [file appendix.tex]

\section*{Appendix}
\subsection*{A.1 Detailed Dataset Description}
\noindent $\bullet$ SNLI \cite{bowman2015large}: Stanford Natural Language Inference is a large-scale dataset for NLI tasks. The goal of this task is to determine whether a hypothesis can be inferred from a premise. This dataset contains 570,152 human-annotated English sentence pairs, out of which 550,152 for training, 10,000 for validation, and 10,000 for testing. These sentence pairs are classified into three categories: entailment, neutral, and contradiction. Several examples from the SNLI dataset are presented in Table \ref{instance}.

\noindent $\bullet$ SNLI-hard \cite{gururangan2018annotation}: This dataset is constructed using the SNLI dataset, but includes only the original training and validation sets. It excludes examples from the original test set that have annotation artifacts. SNLI-hard dataset examples are particularly difficult due to their close relation to specific inference categories such as negation and other linguistic phenomena.

\noindent $\bullet$ SNLI-lexical \cite{glockner2018breaking}: 
This dataset is built on the SNLI and uses the same training and validation sets. However, it adopts a new test set, where the new examples are simpler than the SNLI test set and contains sentences that differ from the training set by only one word. The dataset requires models to understand the relationships between words and is used to evaluate their ability to generalize.

\begin{table*}[ht]
\centering

\resizebox{\textwidth}{!}{%
\begin{tabular}{c|c|c}
\hline
Premise & \begin{tabular}[c]{@{}c@{}}Gold label \\ Annotated label\end{tabular} & Hypothesis \\ \hline
\multirow{2}{*}{Family gathered together in a house enjoy each other company.} &
  Contradiction &
  \multirow{2}{*}{A family is out to eat at a restaurant.} \\ \cline{2-2}
        & C C C E N                                                             &            \\ \hline
\multirow{2}{*}{An older gentleman looks at the cinema while he is building the deck.} &
  Entailment &
  \multirow{2}{*}{\begin{tabular}[c]{@{}c@{}}An older gentleman in overs looks at the cinema \\ while he is building a stained red deck.\end{tabular}} \\ \cline{2-2}
        & E E E N N                                                             &            \\ \hline
\multirow{2}{*}{\begin{tabular}[c]{@{}c@{}}The young Asian woman is using an umbrella, and \\ is in front of a brightly colored patch of flowers.\end{tabular}} &
  Entailment &
  \multirow{2}{*}{A woman is using a large umbrella.} \\ \cline{2-2}
        & E E E N N                                                             &            \\ \hline
\multirow{2}{*}{\begin{tabular}[c]{@{}c@{}}A guy is attempting to perform a skateboard trick\\ while jumping over part of a white building.\end{tabular}} &
  Contradiction &
  \multirow{2}{*}{The skateboard has 8 wheels.} \\ \cline{2-2}
        & C C C N E                                                             &            \\ \hline
\multirow{2}{*}{\begin{tabular}[c]{@{}c@{}}This person looks to be snowboarding on a \\ very small pile of snow on a sunny cold day.\end{tabular}} &
  Entailment &
  \multirow{2}{*}{Young snowboarder sizing up their next jump.} \\ \cline{2-2}
        & E E E N N                                                             &            \\ \hline
\end{tabular}%
}
\caption{Some examples are from the SNLI dataset along with their gold labels and the set of labels (abbreviated) assigned by individual annotators. Our observation reveals that different annotators may have distinct interpretations for identical sentence pairs in the absence of scenarios.}
\label{instance}
\end{table*}

\subsection*{A.2 Descriptions of Baselines}
\noindent (I) We first consider a series of representative \textit{classical sentence-based neural} methods, as detailed below.

\noindent $\bullet$ \textbf{LSTM} \cite{hochreiter1997long}: This model uses two different LSTM networks to encode the premise and hypothesis respectively and then performs classification through a linear layer.

\noindent $\bullet$ \textbf{ESIM} \cite{chen2017enhanced}: It proposes a sequential inference model based on chain LSTM, which explicitly considers the recursive structure in local inference modeling and inference composition, and incorporates syntactic parsing information.

\noindent $\bullet$ \textbf{CAFE} \cite{tay2018compare}: This method first compares and compresses aligned vectors in the designed architecture, and propagates them to the upper layer of the neural network to learn hidden features.

\noindent $\bullet$ \textbf{CSRAN} \cite{tay2018co}: This model introduces a bidirectional alignment mechanism to learn affinity weights in sequence pairs, and uses multi-level attention in stacked recurrent layers, which helps to better learn the matching function between text sequences.

\noindent (II) Besides, we also considered several \textit{pre-trained language model-based} approaches for NLI tasks, which are listed below.

\noindent $\bullet$ \textbf{BERT} \cite{devlin2019bert}: It is a pre-trained language model based on the Transformer architecture and uses bidirectional encoders to learn contextual information, leading to excellent performance across various natural language tasks.

\noindent $\bullet$ \textbf{UERBERT} \cite{xia2021using}: It incorporates prior knowledge into BERT to enhance the performance on downstream tasks by analyzing what task-specific knowledge BERT needs most.

\noindent $\bullet$ \textbf{SemBERT} \cite{zhang2020semantics}: It explicitly integrates contextual information from pre-trained semantic role labeling, which facilitates natural language understanding.

\noindent $\bullet$ \textbf{MT-DNN} \cite{liu2019multi}: This model is based on a pre-trained language model and utilizes a large amount of cross-task data to produce universal representations with beneficial regularization effect that are applicable to new tasks.

\noindent (III) Next, we use two large language models as baselines, which are listed below.

\noindent $\bullet$ \textbf{Bloom-7.1B} \cite{muennighoff2022crosslingual}: It is a decoder-only Transformer language model trained on the ROOTS corpus and shows improved performance following fine-tuning with multi-task prompts.

\noindent $\bullet$ \textbf{Llama2-7B} \cite{touvron2023llama}: It is a  decoder-only large language model, trained on a new combination of data from public datasets. Additionally, it expands the pretraining corpus by 40\%, doubles the model's context length, and utilizes grouped query attention.

\noindent (IV) Furthermore, we introduce several competitive \textit{multimodal} methods, which are stated below. 

\noindent $\bullet$ \textbf{NIC} \cite{vinyals2015show}: It proposes a deep generative model that includes a visual convolutional neural network followed by a language recurrent neural network to simultaneously utilize both language and visual information.

\noindent $\bullet$ \textbf{m-RNN} \cite{mao2014deep}: It proposes a multimodal neural network model, consisting of a recurrent network for sentences and a convolutional network for images, to model the probability distribution of words.

\noindent $\bullet$ \textbf{IEMLRN} \cite{zhang2018image}: It presents a multi-level architecture to leverage information in images and incorporate it with information at different scales in sentences to enhance natural language understanding.

\noindent $\bullet$ \textbf{MIESR} \cite{zhang2019multilevel}: It further extends IEMLRN by simultaneously absorbing both pre-trained coarse-grained features and adaptive fine-grained features from images, achieving ideal results.

\noindent $\bullet$ \textbf{VisualBERT} \cite{li2019visualbert}: It consists of a series of transformer layers that align elements in the input text with relevant regions in the input image through self-attention.

\noindent $\bullet$ \textbf{CLIP} \cite{radford2021learning}: It uses contrastive learning techniques to train the model to understand the semantic relationship between images and texts by aligning them.

\section*{A.3 Implementation Details of Baselines}
For VisualBERT and CLIP, after obtaining the image representations and sentence representations of the training dataset, we train a logistic regression classifier for the NLI task. For Bloom-7.1B and Llama-7B, we perform full-scale fine-tuning using the training data. Specifically, we need to replace the Transformer block at the bottom of the large language model with our proposed method: input $\mathbf{X}$ and $\mathbf{Z}$ to get the representation $\mathbf{R}$ and feed it to the other Transformer blocks. To reduce GPU memory usage, we employ LoRA \cite{hu2021lora} and 4-bit quantization techniques through the Parameter-Efficient Fine-Tuning (PEFT) method provided by Hugging Face. The prompts used for NLI in Bloom-7.1B and Llama2-7B are shown in Table \ref{prompts}. For other baselines, we use the results reported in the original paper for the datasets. If the baselines do not report the results of our used datasets, we carefully select the optimal parameters based on their performance on the validation set and report the final results.

\begin{figure*}

    \centering
    \includegraphics[width=\textwidth]{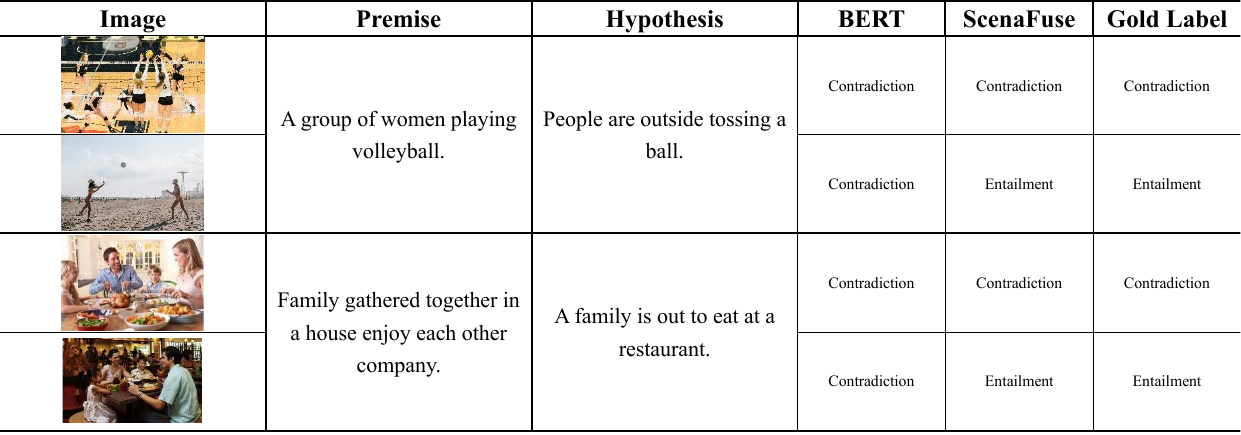}
    \caption{Some examples are accompanied by different scenarios.}
    \label{case}
\end{figure*}

\begin{figure}[ht]

    \centering
    \includegraphics[width=0.45\textwidth]{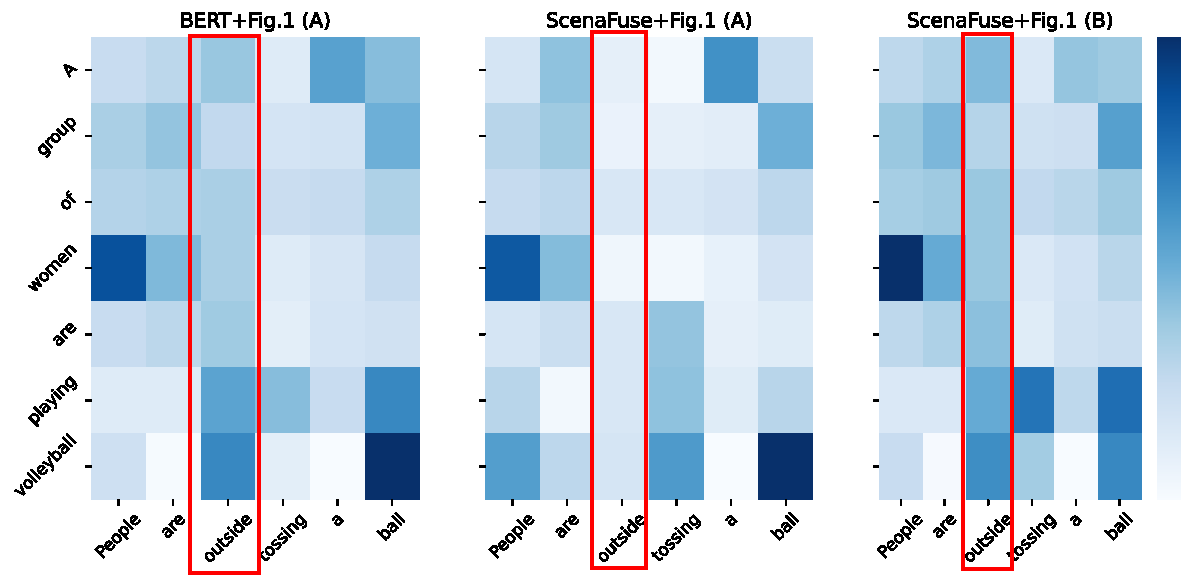}
    \caption{The attention distributions of BERT and ScenaFuse.}
    \label{attention}
\end{figure}

\subsection*{A.4 Case Study}
We conduct qualitative analysis to visually demonstrate the effectiveness of our proposed ScenaFuse. We select some examples from the SNLI dataset, as presented in Fig. \ref{case}. The sentences' semantics conveyed in these examples are ambiguous, and their relationship is entirely opposite when accompanied by different scenarios. Therefore, inferring the semantic relationship from the sentence perspective is challenging. BERT cannot distinguish the variations in the connection between sentence pairs across diverse scenarios and makes predictions based on prior knowledge in the corpus. For example, for the first instance in Fig. \ref{case}, BERT predicts that playing volleyball indoors is more likely, which contradicts the two sentences. However, our proposed ScenaFuse explicitly incorporates visual information through a scenario-guided adapter, aligning the outdoor elements in the second image with the word ``outside'' semantically, thus producing the correct prediction.

Furthermore, we investigate the attention distributions generated by BERT and our ScenaFuse accompanied by different input images using the example in Fig. 1 of the introduction section, shown in Fig. \ref{attention}. In BERT, the word ``outside'' in the hypothesis is assigned higher weights, indicating its significant contribution towards the final contradiction relation inference. However, due to the alignment between the scene information and the ``outside'' in the hypothesis, our ScenaFuse method prioritizes the semantics of the two sentences, with ``people'', ``play'', and ``ball'' having higher weights, leading to entailment inference. When Fig. 1 (B) of the introduction section is used as input, the attention distribution is similar to BERT, with ``outside'' having higher attention values.

\begin{table}[ht]

\resizebox{0.45\textwidth}{!}{%
\begin{tabular}{c|c}
\hline
Dataset                     & Prompts                                                                         \\ \hline
SNLI/SNLI-hard/SNLI-lexical & \begin{tabular}[c]{@{}c@{}}Classify the promise and hypothesis into \\ entailment, neutral, or contradiction.\end{tabular} \\ \hline
\end{tabular}%
}
\caption{Example of prompts used in large language models.}
\label{prompts}
\end{table}

\subsection*{A.5 Further Exploration}

We attempt to replace the image encoder with a pre-trained ViT-large model, and the results are shown in Table \ref{encoder}. We observe that a stronger foundational model can lead to improved performance.

\begin{table}[ht]

\tiny
\centering
\resizebox{0.49\textwidth}{!}{%
\begin{tabular}{c|ccc|ccc|ccc}
\hline
\multirow{2}{*}{Model} & \multicolumn{3}{c|}{SNLI} & \multicolumn{3}{c|}{SNLI-hard} & \multicolumn{3}{c}{SNLI-lexical} \\ \cline{2-10} 
           & Acc   & P     & R     & Acc   & P     & R     & Acc   & P     & R     \\ \hline
ScenaFuse  & 92.16 & 92.06 & 92.12 & 83.25 & 83.16 & 83.20 & 94.05 & 97.07 & 94.04 \\ 
ScenaFuse$_{vit}$ & 92.21 & 92.19 & 92.20 & 83.31 & 83.35 & 83.29 & 94.12 & 97.16 & 94.12 \\ \hline
\end{tabular}%
}
\caption{Results (\%) of different image encoders.}
\label{encoder}
\end{table}

\subsection*{A.6 Discussion Related to Gold Labels}
Since scenarios are not visible during the annotation of the labeled data, introducing scenarios may change the relations between sentences. Would using the original labels still destroy the original model evaluation? According to previous studies \cite{zhang2019multilevel}, they sample three categories evenly from the dataset and invite NLP researchers to relabel them, and finally use \textit{Cohen's} $\kappa$ statistic \cite{warrens2015five} to assess the consistency of the relabeled results with the initial results. The results show that the relabeled data are still reliable. This phenomenon suggests that the introduction of scenarios does not invalidate the evaluation of the model when gold labels are still used. Scenarios have the most significant impact on the neutral relation since they are not visible when labeling the data, and they provide the necessary information to avoid ambiguity or vagueness suffered by the sentence semantics. A neutral hypothesis usually arises by introducing plausible information \cite{gururangan2018annotation}, \textit{e.g.}, \textit{talking outside} to \textit{talking to the teacher outside}, or by replacing approximate descriptions with accurate ones, \textit{e.g.}, \textit{some items} to \textit{five toys}. For the latter case, scenarios provide enough information to distinguish the inferred relations, which can help to avoid such annotated artifacts. Although scenarios do not provide the corresponding information for the former case, they can help the model distinguish plausible information and assign these instances to neutral categories. In other words, although they may change the gold label, it does not invalidate the model evaluation but helps to avoid some annotated artifacts.

\subsection*{A.7 Complexity Analysis}
To further demonstrate the superiority of the model, we perform the following model complexity analysis. In the image-sentence interaction module, we perform two standard transformer layers with time complexity of $O(k^2t+l^2t)$, where \textit{k} and \textit{l} are the lengths of visual blocks and text, and \textit{t} is the dimension of the hidden layer. In the image-sentence fusion module, we perform a total of seven linear transformations, and the time complexity is $O(10t+2lt+t^2)$ in total, which can be reduced to $O(t^2)$. Therefore, the time complexity of our method is $O(k^2t+l^2t+t^2)$, and because $k<l<<t$, the time complexity can be simplified to $O(t^2)$. This is acceptable for the training of the model and does not introduce an intolerable time complexity due to the introduction of the designed module.
